# Supplementary material for: Towards a Robust Detection of Language Model Generated Text: Is ChatGPT that Easy to Detect?
Source: arXiv:2306.05871 source file (2023-06-09)
Supplement: Supplementary file 1 [file appendix.tex]

\section*{Appendix}
